# Supplementary material for: Learning the rules of peptide self-assembly through data mining with large language models
Source: arXiv:2411.05421 source file (2024-11-08)
Supplement: Supplementary file 1 [file si_pages.pdf]

# Supporting Information: Learning the rules of peptide self-assembly through data mining with large language models

**Zhenze Yang<sup>1,2</sup>, Sarah K. Yorke<sup>3</sup>, Tuomas P. J. Knowles<sup>3,4,\*</sup>, and Markus J. Buehler<sup>1,5,6,\*</sup>**

<sup>1</sup>Laboratory for Atomistic and Molecular Mechanics, Department of Civil and Environmental Engineering, Massachusetts Institute of Technology, 77 Massachusetts Ave. Room 1-165, Cambridge, 02139, MA, USA

<sup>2</sup>Department of Materials Science and Engineering, Massachusetts Institute of Technology, 77 Massachusetts Ave., Cambridge, 02139, MA, USA

<sup>3</sup>Yusuf Hamied Department of Chemistry, University of Cambridge, Lensfield Road, Cambridge, CB2 1EW, UK

<sup>4</sup>Cavendish Laboratory, University of Cambridge, J J Thomson Avenue, Cambridge, CB3 0HE, UK

<sup>5</sup>Center for Computational Engineering, Massachusetts Institute of Technology, 77 Massachusetts Ave., Cambridge, 02139, MA, USA

<sup>6</sup>Center for Materials Science and Engineering, Massachusetts Institute of Technology, 77 Massachusetts Ave., Cambridge, 02139, MA, USA

\*mbuehler@mit.edu, tpjk2@cam.ac.uk

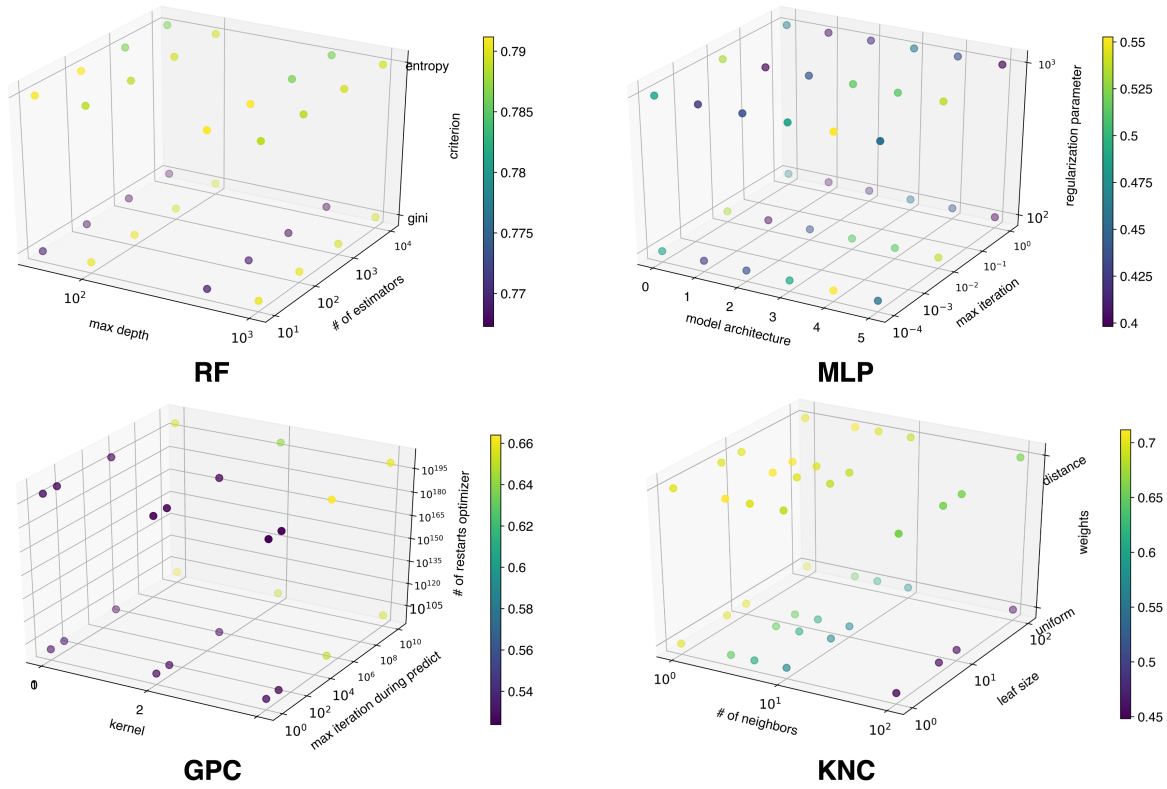

**Figure S1. Hyperparameter grid search for ML algorithms.** The hyperparameter combination for optimal RF model is: 'max depth': 50, '# of estimators': 100, 'criteicon': 'gini'; for optimal MLP classifier is: 'regularization parameter': 0.0001, 'model architecture': (128, 256, 128, 16), 'max iteration': 100; for optimal GPC model is: 'kernel': 2RBF(1), 'max iteration during predict': 100, '# of restarts optimizer': 1; for optimal KNC model is: 'leaf size': 1, '# of neighbors': 3, 'weights': 'distance'.

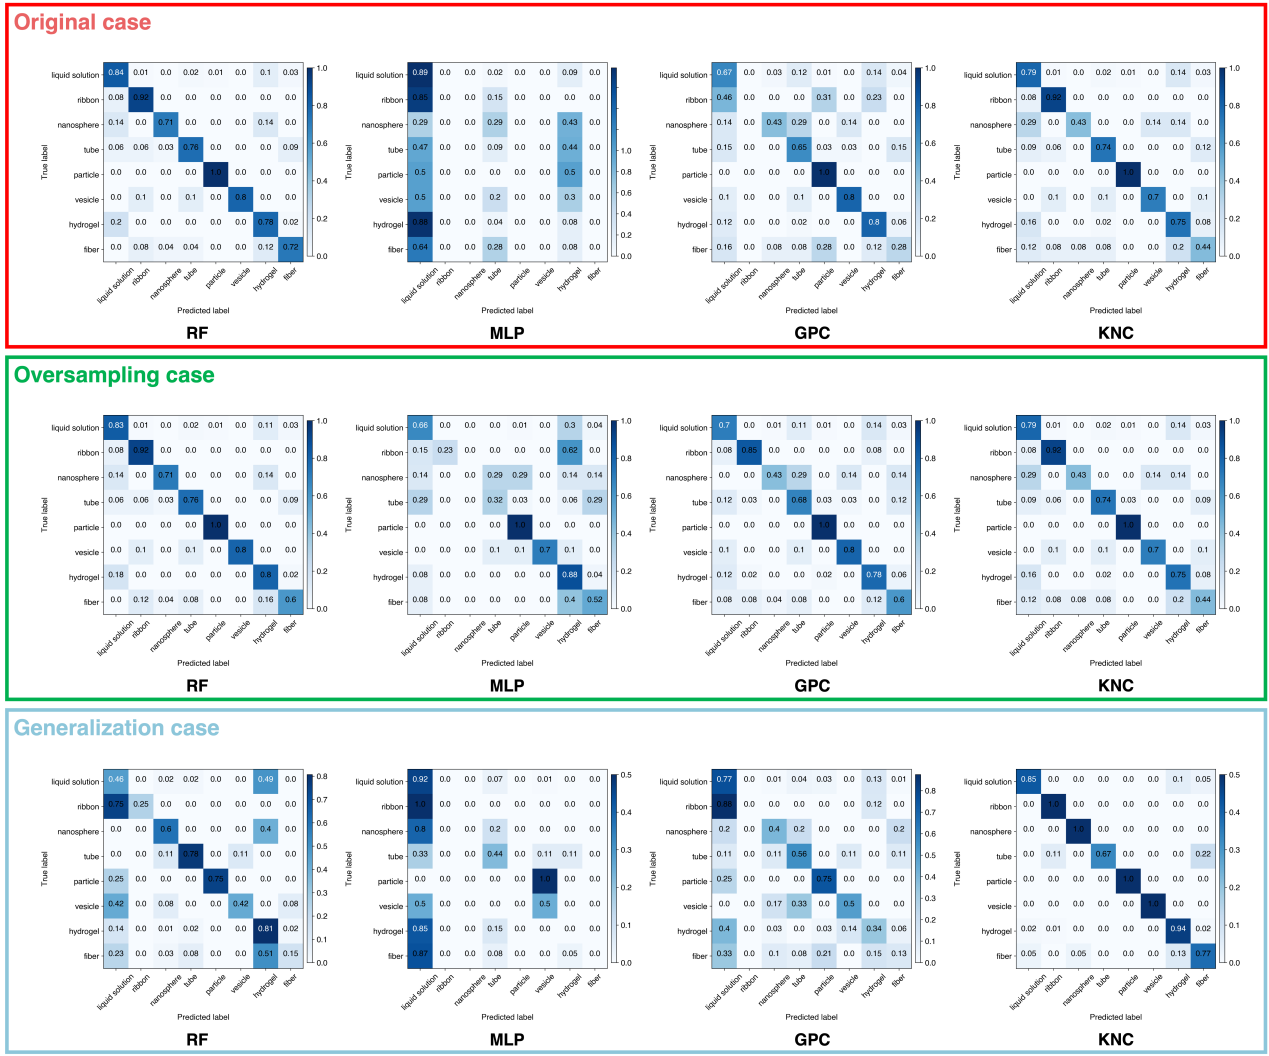

**Figure S2. Confusion matrices.** The confusion matrices, which detail the performance outcomes depicted in Fig. 3b, are arranged in a systematic manner: from top to bottom, they are the original case, the oversampling case, and the generalization case. Horizontally, from left to right, the matrices correspond to the RF, MLP, GPC, and KNC models.

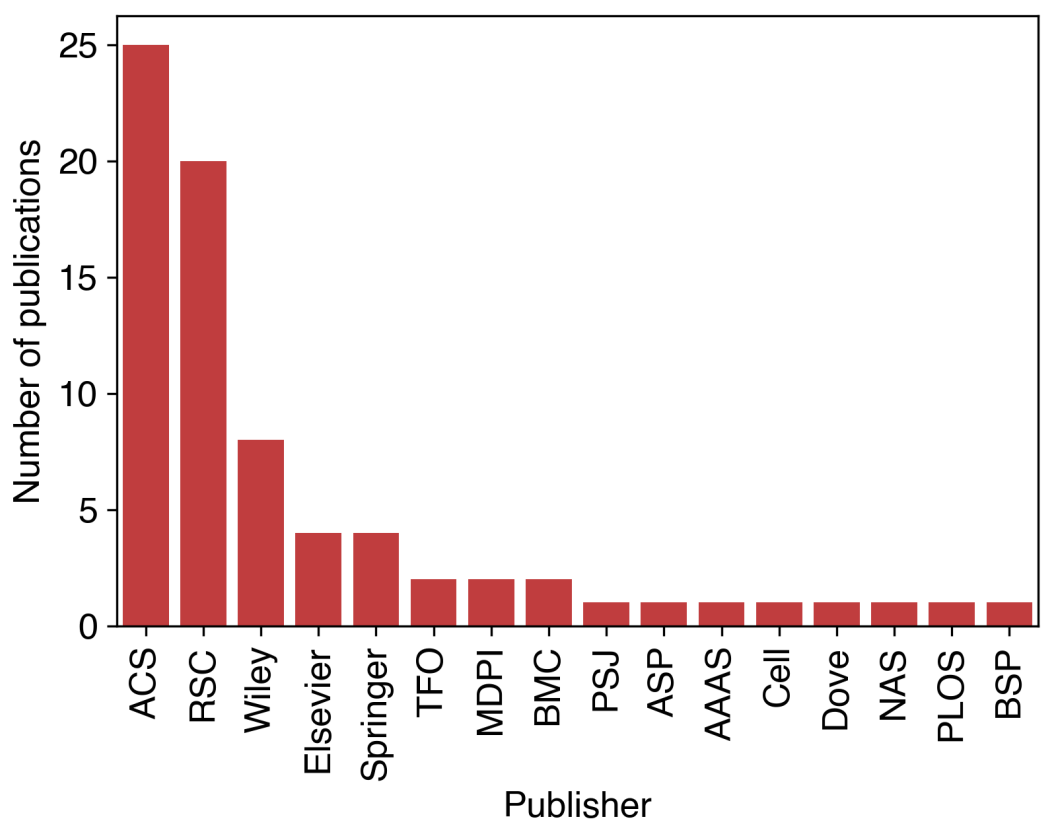

**Figure S3. Publisher information.** We here list the number of publications<sup>1-75</sup> from different journal publishers. The publishers' abbreviations stand for: "ACS" - "American Chemical Society"; "RSC" - "Royal Society of Chemistry"; "TFO" - Taylor & Francis Online; "MDPI" - "Multidisciplinary Digital Publishing Institute"; "BMC" - "BioMed Central"; "PSJ" - "Pharmaceutical Society of Japan"; "ASP" - "American Scientific Publisher"; "AAAS" - "American Association for the Advancement of Science"; "NAS" - "National Academy of Sciences"; "BSP" - "Bentham Science Publishers". Based on the histogram, it is noticeable that the publications are mostly from ACS and RSC publishers.

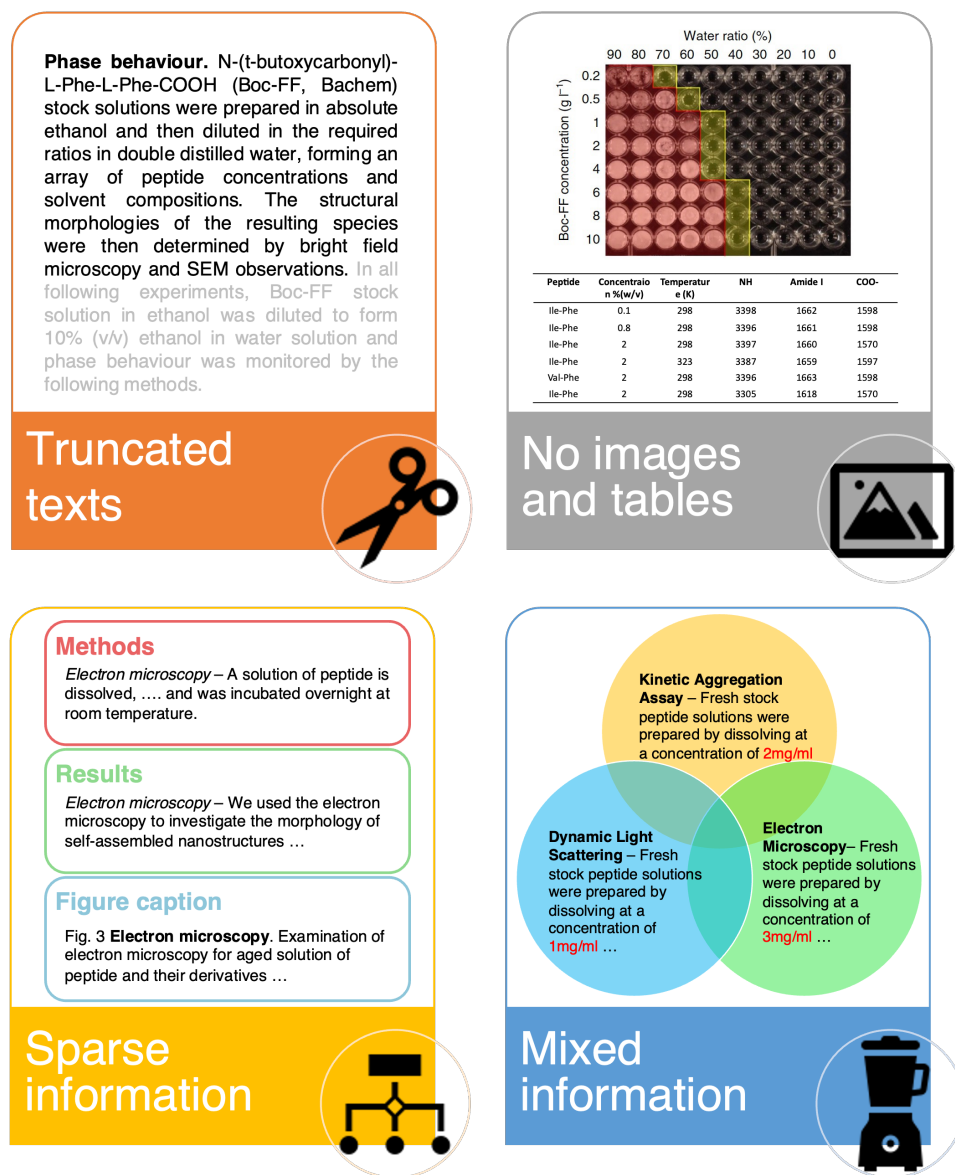

**Figure S4. Limitations of this work.** There are 4 main limitations of current work (from left to right): (1) Due to truncated texts, there can be missing information; (2) No tables or images are included which are frequently used to show self-assembly results; (3) Same group of information can be sparse across the whole text which increases the difficulty of text mining; (4) Information is often mixed. For instance, multiple experiments are utilized to investigate the peptide system which results in multiple sets of experimental conditions. The figure in the limitation related to "No images and tables" is reproduced with permission from Ref.<sup>23</sup>. The table in the same section is created based on the data from Ref.<sup>71</sup>

| Data index | PMID     | Peptide sequence | N-terminal modification | C-terminal modification | Non-terminal modification | Category: peptide/conjugate/mixture | Conjugate partner | Thermal process: heating/cooling |
|------------|----------|------------------|-------------------------|-------------------------|---------------------------|-------------------------------------|-------------------|----------------------------------|
| 1          | 23871602 | FFK              | Acetylation             | Amidation               | None                      | Peptide                             | None              | No                               |
| 2          | 23871602 | FYK              | Acetylation             | Amidation               | None                      | Peptide                             | None              | No                               |
| 3          | 23871602 | YFK              | Acetylation             | Amidation               | None                      | Peptide                             | None              | No                               |
| 4          | 18070345 | FF               | Fmoc                    | None                    | None                      | Peptide                             | None              | No                               |
| 5          | 18070345 | FF               | Fmoc                    | None                    | None                      | Peptide                             | None              | No                               |
| 6          | 18070345 | FF               | Fmoc                    | None                    | None                      | Peptide                             | None              | No                               |
| 7          | 18070345 | FF               | Fmoc                    | None                    | None                      | Peptide                             | None              | No                               |
| Data index | PMID     | Linear/Cyclic    | Solution                | Solvent ratio           | Concentration             | PH                                  | Temperature       | Phase                            |
| 1          | 23871602 | Linear           | HFP/H2O                 | 0.05                    | 1                         | 5.5                                 | 25                | tube                             |
| 2          | 23871602 | Linear           | HFP/H2O                 | 0.05                    | 5                         | 5.5                                 | 25                | fiber                            |
| 3          | 23871602 | Linear           | HFP/H2O                 | 0.05                    | 5                         | 5.5                                 | 25                | fiber                            |
| 4          | 18070345 | Linear           | DMSO/PBS                | 0.05                    | 5.025                     | 7                                   | 37                | none                             |
| 5          | 18070345 | Linear           | DMSO/PBS                | 0.1                     | 10.05                     | 7                                   | 37                | none                             |
| 6          | 18070345 | Linear           | DMSO/PBS                | 0.2                     | 5.025                     | 7                                   | 37                | none                             |
| 7          | 18070345 | Linear           | DMSO/PBS                | 0.4                     | 10.05                     | 7                                   | 37                | none                             |

**Table S1. Data examples.** 7 example data entries from two academic publications (PubMed IDs: 23871602 and 18070345).

| Model | RF              |                             | MLP                       |                                                                                                                                            | GPC                             |                                      | KNC            |                          |
|-------|-----------------|-----------------------------|---------------------------|--------------------------------------------------------------------------------------------------------------------------------------------|---------------------------------|--------------------------------------|----------------|--------------------------|
|       | Hyperparameter  | Values                      | Hyperparameter            | Values                                                                                                                                     | Hyperparameter                  | Values                               | Hyperparameter | Values                   |
| #1    | max depth       | 50,<br>100,<br>500,<br>1000 | model architecture        | (64, 64, 16),<br>(128, 128, 16),<br>(128, 128, 32),<br>(128, 128, 128,<br>16), (128, 256,<br>128, 16), (128,<br>256, 512, 256,<br>128, 16) | kernel                          | RBF(1.0),<br>RBF(10.0),<br>2RBF(1.0) | # of neighbors | 1, 3, 5,<br>10, 100      |
| #2    | # of estimators | 10, 100,<br>1000,<br>10000  | max iteration             | 100, 1000                                                                                                                                  | max iteration<br>during predict | 100, 200                             | leaf size      | 1, 5, 10,<br>100         |
| #3    | criterion       | “gini”,<br>“entropy”        | regularization parameters | 0.0001, 0.01, 1                                                                                                                            | # of restarts<br>optimizer      | 0, 1, 5, 10                          | weights        | “uniform”,<br>“distance” |

**Table S2. Hyperparameter selection.** Hyperparameters for the RF model include: (1) max depth: the maximum depth of the tree; (2) # of estimators: the number of trees in the forest; (3) criterion: the function to measure the quality of a split. For the MLP classifier: (1) model architecture: the sizes of hidden layers as an array; (2) max iteration: maximum number of training iterations; (3) regularization parameters: strength of the L2 regularization term. For the GPC model: (1) kernel: the kernel specifying the covariance function of the Gaussian process; (2) max iteration during predict: the maximum number of iterations in Newton’s method for approximating the posterior during predict; (3) # of restarts optimizer: the number of restarts of the optimizer for finding the kernel’s parameters which maximize the likelihood. For KNC model: (1) # of neighbors: number of neighbors used for queries; (2) leaf size: leaf size passed to BallTree or KDTree; (3) weights: weight function category.

| Relevant entity   | Key words                                                                                                                                                                                                                                                                                                                                                                                                                                                                                                                                                                                                                                                                                                                                                                                                                                                                                                                                                                                                                                                                                                                                                                                                                                                                                                                                                                                                                                                             |
|-------------------|-----------------------------------------------------------------------------------------------------------------------------------------------------------------------------------------------------------------------------------------------------------------------------------------------------------------------------------------------------------------------------------------------------------------------------------------------------------------------------------------------------------------------------------------------------------------------------------------------------------------------------------------------------------------------------------------------------------------------------------------------------------------------------------------------------------------------------------------------------------------------------------------------------------------------------------------------------------------------------------------------------------------------------------------------------------------------------------------------------------------------------------------------------------------------------------------------------------------------------------------------------------------------------------------------------------------------------------------------------------------------------------------------------------------------------------------------------------------------|
| Phase             | "gel", "fibr", "lamellar", "flower", "fiber", "filament", "spher", "microcrystal", "tube", "rod", "plate", "flake", "particle", "vesic", "ribbon", "bead", "sheet", "tape", "belt", "film"                                                                                                                                                                                                                                                                                                                                                                                                                                                                                                                                                                                                                                                                                                                                                                                                                                                                                                                                                                                                                                                                                                                                                                                                                                                                            |
| PH, Concentration | dissolve", "dilute", "elute", "wash", "dispers", "soluble", "mixed", "added", "pH", "prepare", "concentration", "mM", "μM", "μM", "μL", "μL", "μg", "μg", "g/ml", "gymL", "mg/ml", "mgymL", "g/L", "gyL", "kg/L", "kgL", "w/w", "w/v", "v/v"                                                                                                                                                                                                                                                                                                                                                                                                                                                                                                                                                                                                                                                                                                                                                                                                                                                                                                                                                                                                                                                                                                                                                                                                                          |
| Solution          | "acetic acid", "acetone", "acetonitrile", "acetyl acetone", "2-aminoethanol", "aniline", "anisole", "benzene", "benzonitrile", "benzyl alcohol", "1-butanol", "2-butanol", "i-butanol", "2-butanone", "t-butyl alcohol", "carbon disulfide", "carbon tetrachloride", "chlorobenzene", "chloroform", "cyclohexane", "cyclohexanol", "cyclohexanone", "di-n-butylphthalate", "1,1-dichloroethane", "1,2-dichloroethane", "diethylamine", "diethylene glycol", "diglyme", "dimethoxyethane", "glyme", "N,N-dimethylaniline", "dimethylformamide", "DMF", "dimethylphthalate", "dimethylsulfoxide", "DMSO", "dioxane", "ethanol", "ether", "ethyl acetate", "ethyl acetoacetate", "ethyl benzoate", "ethylene glycol", "glycerin", "heptane", "1-heptanol", "hexane", "1-hexanol", "methanol", "methyl acetate", "methyl t-butyl ether", "MTBE", "methylene chloride", "1-octanol", "pentane", "1-pentanol", "2-pentanol", "3-pentanol", "2-pentanone", "3-pentanone", "1-propanol", "2-propanol", "pyridine", "tetrahydrofuran", "THF", "toluene", "water", "H2O", "D2O", "o-xylene", "p-xylene", "m-xylene", "heavy water", "water, heavy", "phosphate-buffered saline", "PBS", "sodium phosphate", "hexafluoro-2-propanol", "HFP", "HFIP", "phosphate buffer", "NaOH", "NaCl", "HCl", "glucono delta-lactone", "GdL", "dichloromethane", "1,3-butanediol", "dimethyl carbonate", "pyrimidine", "pyridine", "mesitylene", "octane", "decane", "isopropanol", "glycine". |

**Table S3. Key words for paragraph collection.** For each paragraph in the text, it is kept if any of the specified keywords are found within it; otherwise, the paragraph is removed.

| Limitations                                                                                                                                                                                                                                                                                                       | Solutions                                                                                                                                                                                                                                                                                  |
|-------------------------------------------------------------------------------------------------------------------------------------------------------------------------------------------------------------------------------------------------------------------------------------------------------------------|--------------------------------------------------------------------------------------------------------------------------------------------------------------------------------------------------------------------------------------------------------------------------------------------|
| Given the limit of token numbers, we trunk the full texts of academic publications which can eliminate important information from the text.                                                                                                                                                                       | We believe that as training and fine-tuning LLMs become widely accessible to researchers, this issue will be effectively mitigated.                                                                                                                                                        |
| We only keep the text of publications for data mining. However, figures, tables and videos often contain essential information about self-assembly results.                                                                                                                                                       | Multimodal LLMs are capable of simultaneously processing text, images, and videos, offering a comprehensive and integrated approach to literature mining.                                                                                                                                  |
| The experimental information is often distribute sparsely throughout the full text. For instance, the same group of information, such as observations from electron microscopic examination (see Fig. S4), may be dispersed across various sections of a paper, including Methods, Results, and figure captions.  | A potential solution is to group these relevant information by matching key words using another LLMs during the initial stage of preprocessing. Consequently, the LLMs employed for text mining can more effectively learn from text that is originally scattered throughout the document. |
| There are often frequent occurrence of multiple experiments conducted on the same peptide system to explore its morphology, composition, and properties. This result in a mixture of target information we aim to extract, involving multiple sets of experimental conditions which confuses the LLMs we utilize. | We propose the inclusion of the experimental method as an additional entity for information extraction. This approach facilitates the clearer separation of intertwined information.                                                                                                       |

**Table S4. Limitations and solutions.** Limitations of current literature mining approach and potential solutions for the future works.

## References

1. Kurbasic, M., Romano, C. D., Garcia, A. M., Kralj, S. & Marchesan, S. Assembly of a tripeptide and anti-inflammatory drugs into supramolecular hydrogels for sustained release. *Gels* **3**, DOI: [10.3390/gels3030029](https://doi.org/10.3390/gels3030029) (2017).
2. Xing, Q. G. *et al.* Aromatic Motifs Dictate Nanohelix Handedness of Tripeptides. *ACS NANO* **12**, 12305–12314, DOI: [10.1021/acs.nano.8b06173](https://doi.org/10.1021/acs.nano.8b06173) (2018).
3. Li, Q. *et al.* Peptide-templated synthesis of tio<sub>2</sub> nanofibers with tunable photocatalytic activity. *Chem. A Eur. J.* **24**, 18123–18129, DOI: <https://doi.org/10.1002/chem.201804514> (2018). <https://chemistry-europe.onlinelibrary.wiley.com/doi/pdf/10.1002/chem.201804514>.
4. Tao, K. *et al.* Quantum confined peptide assemblies with tunable visible to near-infrared spectral range. *Nat. Commun.* **1–11**, DOI: [10.1038/s41467-018-05568-9](https://doi.org/10.1038/s41467-018-05568-9) (2018).
5. Dudukovic, N. A., Hudson, B. C., Paravastu, A. K. & Zukoski, C. F. Self-assembly pathways and polymorphism in peptide-based nanostructures. *Nanoscale* **10**, 1508–1516, DOI: [10.1039/c7nr06724k](https://doi.org/10.1039/c7nr06724k) (2018).
6. Ishikawa, M. S., Busch, C., Motzkus, M., Martinho, H. & Buckup, T. Two-step kinetic model of the self-assembly mechanism for diphenylalanine micro/nanotube formation. *Phys. Chem. Chem. Phys.* **19**, 31647–31654, DOI: [10.1039/c7cp06611b](https://doi.org/10.1039/c7cp06611b) (2017).
7. Mason, T. O. *et al.* Thermodynamics of Polypeptide Supramolecular Assembly in the Short-Chain Limit. *J. Am. Chem. Soc.* **139**, 16134–16142, DOI: [10.1021/jacs.7b00229](https://doi.org/10.1021/jacs.7b00229) (2017).
8. Ghosh, M. *et al.* Arginine-Presenting Peptide Hydrogels Decorated with Hydroxyapatite as Biomimetic Scaffolds for Bone Regeneration. *Biomacromolecules* **18**, 3541–3550, DOI: [10.1021/acs.biomac.7b00876](https://doi.org/10.1021/acs.biomac.7b00876) (2017).
9. Abul-Haija, Y. M., Scott, G. G., Sahoo, J. K., Tuttle, T. & Ulijn, R. V. Cooperative, ion-sensitive co-assembly of tripeptide hydrogels. *Chem. Commun.* **53**, 9562–9565, DOI: [10.1039/c7cc04796g](https://doi.org/10.1039/c7cc04796g) (2017).
10. Yang, X., Wang, Y., Qi, W., Su, R. & He, Z. Bioorganometallic ferrocene-tripeptide nanoemulsions. *Nanoscale* **9**, 15323–15331, DOI: [10.1039/c7nr03932h](https://doi.org/10.1039/c7nr03932h) (2017).
11. Garcia, A. M., Kurbasic, M., Kralj, S., Melchionna, M. & Marchesan, S. A biocatalytic and thermoreversible hydrogel from a histidine-containing tripeptide. *Chem. Commun.* **53**, 8110–8113, DOI: [10.1039/c7cc03371k](https://doi.org/10.1039/c7cc03371k) (2017).
12. Subbalakshmi, C., Basak, P. & Nagaraj, R. Self-assembly of t-butyloxycarbonyl protected dipeptide methyl esters composed of leucine, isoleucine, and valine into highly organized structures from alcohol and aqueous alcohol mixtures. *Biopolymers* **108**, DOI: [10.1002/bip.23033](https://doi.org/10.1002/bip.23033) (2017).
13. Sahoo, J. K., Nazareth, C., Vandenberg, M. A. & Webber, M. J. Self-assembly of amphiphilic tripeptides with sequence-dependent nanostructure. *Biomater. Sci.* **5**, 1526–1530, DOI: [10.1039/c7bm00304h](https://doi.org/10.1039/c7bm00304h) (2017).
14. Liu, X. *et al.* Transformation of Dipeptide-Based Organogels into Chiral Crystals by Cryogenic Treatment. *Angewandte Chemie - Int. Ed.* **56**, 2660–2663, DOI: [10.1002/anie.201612024](https://doi.org/10.1002/anie.201612024) (2017).
15. Moitra, P., Subramanian, Y. & Bhattacharya, S. Concentration Dependent Self-Assembly of TrK-NGF Receptor Derived Tripeptide: New Insights from Experiment and Computer Simulations. *J. Phys. Chem. B* **121**, 815–824, DOI: [10.1021/acs.jpcc.6b10511](https://doi.org/10.1021/acs.jpcc.6b10511) (2017).
16. Pospišil, T. *et al.* Synthesis, characterization and: In vitro biocompatibility assessment of a novel tripeptide hydrogelator, as a promising scaffold for tissue engineering applications. *Biomater. Sci.* **4**, 1412–1416, DOI: [10.1039/c6bm00287k](https://doi.org/10.1039/c6bm00287k) (2016).
17. Bhardwaj, I., Jha, D., Admane, P., Panda, A. K. & Haridas, V. Self-assembling tryptophan-based designer peptides as intracellular delivery vehicles. *Bioorganic Medicinal Chem. Lett.* **26**, 672–676, DOI: [10.1016/j.bmcl.2015.11.041](https://doi.org/10.1016/j.bmcl.2015.11.041) (2016).
18. Pappas, C. G. *et al.* Alignment of nanostructured tripeptide gels by directional ultrasonication. *Chem. Commun.* **51**, 8465–8468, DOI: [10.1039/c5cc02049b](https://doi.org/10.1039/c5cc02049b) (2015).
19. Yadav, S. *et al.* Vitamin E–TPGS Stabilized Self-Assembled Tripeptide Nanostructures for Drug Delivery, DOI: <http://dx.doi.org/10.2174/1568026615666150330111348> (2015).
20. Xie, Y. *et al.* Electrostatic and aromatic interaction-directed supramolecular self-assembly of a designed fmoc-tripeptide into helical nanoribbons. *Langmuir* **31**, 2885–2894, DOI: [10.1021/la504757c](https://doi.org/10.1021/la504757c) (2015).
21. Nigg, J. T. Aligning 3D nanofibrous networks from self-assembled phenylalanine nanofibers. *Bone* **23**, 1–7, DOI: [10.1039/C4RA13159B](https://doi.org/10.1039/C4RA13159B). *Aligning* (2008). [NIHMS150003](https://pubmed.ncbi.nlm.nih.gov/150003/).
22. Frederix, P. W. *et al.* Exploring the sequence space for (tri-)peptide self-assembly to design and discover new hydrogels. *Nat. Chem.* **7**, 30–37, DOI: [10.1038/nchem.2122](https://doi.org/10.1038/nchem.2122) (2015).

23. Levin, A. *et al.* Ostwalds rule of stages governs structural transitions and morphology of dipeptide supramolecular polymers. *Nat. Commun.* **5**, DOI: [10.1038/ncomms6219](https://doi.org/10.1038/ncomms6219) (2014).
24. Liu, Y. H. *et al.* Electroactive organic dye incorporating dipeptides in the formation of self-assembled nanofibrous hydrogels. *Bioconjugate Chem.* **25**, 1794–1800, DOI: [10.1021/bc500299c](https://doi.org/10.1021/bc500299c) (2014).
25. Laverty, G. *et al.* Ultrashort cationic naphthalene-derived self-assembled peptides as antimicrobial nanomaterials. *Biomacromolecules* **15**, 3429–3439, DOI: [10.1021/bm500981y](https://doi.org/10.1021/bm500981y) (2014).
26. Smadbeck, J. *et al.* De Novo Design and Experimental Characterization of Ultrashort Self-Associating Peptides. *PLoS Comput. Biol.* **10**, DOI: [10.1371/journal.pcbi.1003718](https://doi.org/10.1371/journal.pcbi.1003718) (2014).
27. Bai, S. *et al.* Stable emulsions formed by self-assembly of interfacial networks of dipeptide derivatives. *ACS Nano* **8**, 7005–7013, DOI: [10.1021/nn501909j](https://doi.org/10.1021/nn501909j) (2014).
28. Handelman, A., Natan, A. & Rosenman, G. Structural and optical properties of short peptides: Nanotubes-to- nanofibers phase transformation. *J. Pept. Sci.* **20**, 487–493, DOI: [10.1002/psc.2661](https://doi.org/10.1002/psc.2661) (2014).
29. Gour, N. *et al.* Label-free, optical sensing of the supramolecular assembly into fibrils of a ditryptophan–DNA hybrid. *Chem. Commun.* **50**, 6863–6865, DOI: [10.1039/c4cc02631d](https://doi.org/10.1039/c4cc02631d) (2014).
30. Eckes, K. M., Mu, X., Ruehle, M. A., Ren, P. & Suggs, L. J.  $\beta$  Sheets not required: Combined experimental and computational studies of self-assembly and gelation of the ester-containing analogue of an Fmoc-Dipeptide Hydrogelator. *Langmuir* **30**, 5287–5296, DOI: [10.1021/la500679b](https://doi.org/10.1021/la500679b) (2014).
31. Marchesan, S. *et al.* Chirality effects at each amino acid position on tripeptide self-assembly into hydrogel biomaterials. *Nanoscale* **6**, 5172–5180, DOI: [10.1039/c3nr06752a](https://doi.org/10.1039/c3nr06752a) (2014).
32. Ghosh, S. & Banerjee, A. for Sustained Release of Drugs. *Langmuir* **30**, 929–936 (2014).
33. Moitra, P., Kumar, K., Kondaiah, P. & Bhattacharya, S. Efficacious anticancer drug delivery mediated by a pH-sensitive self-assembly of a conserved tripeptide derived from tyrosine kinase NGF receptor. *Angewandte Chemie - Int. Ed.* **53**, 1113–1117, DOI: [10.1002/anie.201307247](https://doi.org/10.1002/anie.201307247) (2014).
34. Tang, C., Ulijn, R. V. & Saiani, A. Self-assembly and gelation properties of glycine/leucine Fmoc-dipeptides. *Eur. Phys. J. E* **36**, DOI: [10.1140/epje/i2013-13111-3](https://doi.org/10.1140/epje/i2013-13111-3) (2013).
35. Li, Y., Li, B., Fu, Y., Lin, S. & Yang, Y. Solvent-induced handedness inversion of dipeptide sodium salts derived from alanine. *Langmuir* **29**, 9721–9726, DOI: [10.1021/la402174w](https://doi.org/10.1021/la402174w) (2013).
36. Kleinsmann, A. J. & Nachtsheim, B. J. Phenylalanine-containing cyclic dipeptides – the lowest molecular weight hydrogelators based on unmodified proteinogenic amino acids. *Chem. Commun.* **49**, 7818–7820, DOI: [10.1039/c3cc44110e](https://doi.org/10.1039/c3cc44110e) (2013).
37. Cao, M., Cao, C., Zhang, L., Xia, D. & Xu, H. Tuning of peptide assembly through force balance adjustment. *J. Colloid Interface Sci.* **407**, 287–295, DOI: [10.1016/j.jcis.2013.06.051](https://doi.org/10.1016/j.jcis.2013.06.051) (2013).
38. Erdogan, H., Sakalak, H., Yavuz, M. S. & Demirel, G. Laser-triggered degelation control of gold nanoparticle embedded peptide organogels. *Langmuir* **29**, 6975–6982, DOI: [10.1021/la401300u](https://doi.org/10.1021/la401300u) (2013).
39. Panda, J. J., Varshney, A. & Chauhan, V. S. Self-assembled nanoparticles based on modified cationic dipeptides and DNA: Novel systems for gene delivery. *J. Nanobiotechnology* **11**, 1, DOI: [10.1186/1477-3155-11-18](https://doi.org/10.1186/1477-3155-11-18) (2013).
40. Marchesan, S. *et al.* Self-assembly of ciprofloxacin and a tripeptide into an antimicrobial nanostructured hydrogel. *Biomaterials* **34**, 3678–3687, DOI: [10.1016/j.biomaterials.2013.01.096](https://doi.org/10.1016/j.biomaterials.2013.01.096) (2013).
41. Panda, J. J. *et al.* Modified dipeptide-based nanoparticles: Vehicles for targeted tumor drug delivery. *Nanomedicine* **8**, 1927–1942, DOI: [10.2217/nnm.12.201](https://doi.org/10.2217/nnm.12.201) (2013).
42. Dudukovic, N. A. & Zukoski, C. F. Gelation of Fmoc-diphenylalanine is a first order phase transition. *Soft Matter* **11**, 7663–7673, DOI: [10.1039/c5sm01399b](https://doi.org/10.1039/c5sm01399b) (2015).
43. Lakshmanan, A. *et al.* Aliphatic peptides show similar self-assembly to amyloid core sequences, challenging the importance of aromatic interactions in amyloidosis. *PROCEEDINGS OF THE NATIONAL ACADEMY OF SCIENCES OF THE UNITED STATES OF AMERICA* **110**, 519–524, DOI: [10.1073/pnas.1217742110](https://doi.org/10.1073/pnas.1217742110) (2013).
44. Zheng, W. *et al.* Surface-induced hydrogelation inhibits platelet aggregation. *J. Am. Chem. Soc.* **135**, 266–271, DOI: [10.1021/ja308690y](https://doi.org/10.1021/ja308690y) (2013).
45. Mu, X. *et al.* Experimental and Computational Studies Reveal An Alternative. *Biomacromolecules* **18**, 1199–1216, DOI: [10.1021/bm301007r](https://doi.org/10.1021/bm301007r). Experimental (2013). NIHMS150003.

46. Nanda, J., Adhikari, B., Basak, S. & Banerjee, A. Formation of hybrid hydrogels consisting of tripeptide and different silver nanoparticle-capped ligands: Modulation of the mechanical strength of gel phase materials. *J. Phys. Chem. B* **116**, 12235–12244, DOI: [10.1021/jp306262t](https://doi.org/10.1021/jp306262t) (2012).
47. Marchesan, S. *et al.* Unzipping the role of chirality in nanoscale self-assembly of tripeptide hydrogels. *Nanoscale* **4**, 6752–6760, DOI: [10.1039/c2nr32006a](https://doi.org/10.1039/c2nr32006a) (2012).
48. Alam, S., Panda, J. J. & Chauhan, V. S. Novel dipeptide nanoparticles for effective curcumin delivery. *Int. J. Nanomedicine* **7**, 4207–4222, DOI: [10.2147/IJN.S33015](https://doi.org/10.2147/IJN.S33015) (2012).
49. Panda, J. J. *et al.* Designed peptides as model self-assembling nanosystems: Characterization and potential biomedical applications. *Ther. Deliv.* **2**, 193–204, DOI: [10.4155/tde.10.93](https://doi.org/10.4155/tde.10.93) (2011).
50. Subbalakshmi, C., Manorama, S. V. & Nagaraj, R. Self-assembly of short peptides composed of only aliphatic amino acids and a combination of aromatic and aliphatic amino acids. *JOURNAL OF PEPTIDE SCIENCE* **18**, 283–292, DOI: [10.1002/psc.2395](https://doi.org/10.1002/psc.2395) (2012).
51. Marchesan, S., Easton, C. D., Kushkaki, F., Waddington, L. & Hartley, P. G. Tripeptide self-assembled hydrogels: Unexpected twists of chirality. *Chem. Commun.* **48**, 2195–2197, DOI: [10.1039/c2cc16609g](https://doi.org/10.1039/c2cc16609g) (2012).
52. Berillo, D., Mattiasson, B., Galaev, I. Y. & Kirsebom, H. Formation of macroporous self-assembled hydrogels through cryogelation of Fmoc-Phe-Phe. *J. Colloid Interface Sci.* **368**, 226–230, DOI: [10.1016/j.jcis.2011.11.006](https://doi.org/10.1016/j.jcis.2011.11.006) (2012).
53. Lakshmanan, A. & Hauser, C. A. Ultrasmall peptides self-assemble into diverse nanostructures: Morphological evaluation and potential implications anupama. *Int. J. Mol. Sci.* **12**, 5736–5746, DOI: [10.3390/ijms12095736](https://doi.org/10.3390/ijms12095736) (2011).
54. Chen, L. *et al.* Salt-induced hydrogelation of functionalised-dipeptides at high pH. *Chem. Commun.* **47**, 12071–12073, DOI: [10.1039/c1cc15474e](https://doi.org/10.1039/c1cc15474e) (2011).
55. Tang, C., Ulijn, R. V. & Saiani, A. Effect of glycine substitution on Fmoc-diphenylalanine self-assembly and gelation properties. *Langmuir* **27**, 14438–14449, DOI: [10.1021/la202113j](https://doi.org/10.1021/la202113j) (2011).
56. Naskar, J., Roy, S., Joardar, A., Das, S. & Banerjee, A. Self-assembling dipeptide-based nontoxic vesicles as carriers for drugs and other biologically important molecules. *Org. Biomol. Chem.* **9**, 6610–6615, DOI: [10.1039/c1ob05757j](https://doi.org/10.1039/c1ob05757j) (2011).
57. Mishra, A. & Chauhan, V. S. Probing the role of aromaticity in the design of dipeptide based nanostructures. *Nanoscale* **3**, 945–949, DOI: [10.1039/c0nr00691b](https://doi.org/10.1039/c0nr00691b) (2011).
58. Chen, L., Revel, S., Morris, K., C. Serpell, L. & Adams, D. J. Effect of molecular structure on the properties of naphthalene-dipeptide hydrogelators. *Langmuir* **26**, 13466–13471, DOI: [10.1021/la102059x](https://doi.org/10.1021/la102059x) (2010).
59. Chen, L., Revel, S., Morris, K. & Adams, D. J. Energy transfer in self-assembled dipeptide hydrogels. *Chem. Commun.* **46**, 4267–4269, DOI: [10.1039/c003052j](https://doi.org/10.1039/c003052j) (2010).
60. Azuma, E., Kuramochi, K. & Tsubaki, K. Development of supramolecular organo-gel based on tripeptide skeletons. *Chem. Pharm. Bull.* **58**, 680–684, DOI: [10.1248/cpb.58.680](https://doi.org/10.1248/cpb.58.680) (2010).
61. Biswas, K. & Rao, C. N. Nanostructured peptide fibrils formed at the organic-aqueous interface and their use as templates to prepare inorganic nanostructures. *ACS Appl. Mater. Interfaces* **1**, 811–815, DOI: [10.1021/am800233s](https://doi.org/10.1021/am800233s) (2009).
62. Demirel, G., Malvadkar, N. & Demirel, M. C. Control of protein adsorption onto core-shell tubular and vesicular structures of diphenylalanine/parylene. *Langmuir* **26**, 1460–1463, DOI: [10.1021/la903571y](https://doi.org/10.1021/la903571y) (2010).
63. Chen, L. *et al.* Self-assembly mechanism for a naphthalene-dipeptide leading to hydrogelation. *Langmuir* **26**, 5232–5242, DOI: [10.1021/la903694a](https://doi.org/10.1021/la903694a) (2010).
64. Orbach, R. *et al.* Self-assembled Fmoc-peptides as a platform for the formation of nanostructures and hydrogels. *Biomacromolecules* **10**, 2646–2651, DOI: [10.1021/bm900584m](https://doi.org/10.1021/bm900584m) (2009).
65. Han, T. H., Park, J. S., Oh, J. K. & Kim, S. O. Morphology control of one-dimensional peptide nanostructures. *J. Nanosci. Nanotechnol.* **8**, 5547–5550, DOI: [10.1166/jnn.2008.1311](https://doi.org/10.1166/jnn.2008.1311) (2008).
66. Mishra, A., Panda, J. J., Basu, A. & Chauhan, V. S. Nanovesicles based on self-assembly of conformationally constrained aromatic residue containing amphiphilic dipeptides. *Langmuir* **24**, 4571–4576, DOI: [10.1021/la7034533](https://doi.org/10.1021/la7034533) (2008).
67. Liebmann, T., Rydholm, S., Akpe, V. & Brismar, H. Self-assembling Fmoc dipeptide hydrogel for in situ 3D cell culturing. *BMC Biotechnol.* **7**, 88, DOI: [10.1186/1472-6750-7-88](https://doi.org/10.1186/1472-6750-7-88) (2007).
68. Mitra, R. N., Das, D., Roy, S. & Das, P. K. Structure and properties of low molecular weight amphiphilic peptide hydrogelators. *J. Phys. Chem. B* **111**, 14107–14113, DOI: [10.1021/jp076495x](https://doi.org/10.1021/jp076495x) (2007).

69. Adler-Abramovich, L. & Gazit, E. Controlled patterning of peptide nanotubes and nanospheres using inkjet printing technology. *J. Pept. Sci.* **14**, 217–223, DOI: [10.1002/psc.963](https://doi.org/10.1002/psc.963) (2008).
70. Yan, X. *et al.* Transition of cationic dipeptide nanotubes into vesicles and oligonucleotide delivery. *Angewandte Chemie - Int. Ed.* **46**, 2431–2434, DOI: [10.1002/anie.200603387](https://doi.org/10.1002/anie.200603387) (2007).
71. De Groot, N. S., Parella, T., Aviles, F. X., Vendrell, J. & Ventura, S. Ile-Phe dipeptide self-assembly: Clues to amyloid formation. *Biophys. J.* **92**, 1732–1741, DOI: [10.1529/biophysj.106.096677](https://doi.org/10.1529/biophysj.106.096677) (2007).
72. Sedman, V. L., Adler-Abramovich, L., Allen, S., Gazit, E. & Tendler, S. J. Direct observation of the release of phenylalanine from diphenylalanine nanotubes. *J. Am. Chem. Soc.* **128**, 6903–6908, DOI: [10.1021/ja060358g](https://doi.org/10.1021/ja060358g) (2006).
73. Adler-Abramovich, L. *et al.* Thermal and chemical stability of diphenylalanine peptide nanotubes: Implications for nanotechnological applications. *Langmuir* **22**, 1313–1320, DOI: [10.1021/la052409d](https://doi.org/10.1021/la052409d) (2006).
74. Reches, M. & Gazit, E. Casting metal nanowires within discrete self-assembled peptide nanotubes. *Science* **300**, 625–627, DOI: [10.1126/science.1082387](https://doi.org/10.1126/science.1082387) (2003).
75. Mukai, M. *et al.* A hydro/organo/hybrid gelator: A peptide lipid with turning aspartame head groups. *J. Colloid Interface Sci.* **395**, 154–160, DOI: <https://doi.org/10.1016/j.jcis.2012.12.060> (2013).
